# Supplementary material for: Optimizing Trajectory-Trees in Belief Space: An Application from Model Predictive Control to Task and Motion Planning
Source: arXiv:2605.01860 source file (2026-08-09)
Supplement: Supplementary file 1 [file 5_proof_appendix_full.tex]

\subsection{Scope of the Proof}
The following section provides a proof of convergence and optimality of the \textit{Distributed Augmented Lagrangian} algorithm under the following assumptions:
\begin{itemize}
\item Presence of equality constraints, but no inequality contraints
\item Full overlap of the optimization problems. This implies that the sub-optimization variables have the same dimensions
\end{itemize}
Under those assumptions, we can formally define the optimization problem.

Let $z_i \in \mathbb{R}^{n}, i \in [1..N]$, $f_i:\mathbb{R}^{n} \rightarrow \mathbb{R}, i \in [1..N]$ be $N$ derivable cost functions, and $h_i:\mathbb{R}^{n} \rightarrow \mathbb{R}^m, , i \in [1..N]$ be $N$ derivable equality constraints vector-valued functions.
\begin{definition} 
We define the \textit{Distributed Augmented Lagrangian} optimization objective~as:
\begin{subequations}
\begin{align}  
  \min_{\tilde{z}, z_i}&{
  \ \sum_i{c_i(z_i)} \label{eq:consensus_admm_cost}
  },\\
 &\text{s.t.} \notag \\
 & h_i(z_i) = 0, \label{eq:consensus_h_constraint}\\
 & z_i = \tilde{z}, \label{eq:consensus_z_admm_constraint}
\end{align}
\end{subequations}
where $\tilde{z} \in \mathbb{R}^n$ is an auxilary optimization variable use to define an equality constraints stating that all $z_i$ should reach a consensus at the optimum.
\end{definition}
For a given $i$, we call the triple $(c_i, h_i, z_i)$ a subproblem.
\begin{definition} 
We define the \textit{Distributed Augmented Lagrangian}~corresponding to the $i\textsuperscript{th}$ subproblem as:
\begin{align} 
  L_{i, \nu, \rho}(\tilde{z}, z_i, \kappa_i, \eta_i) =&
  c_i(z_i) \label{eq:dec_lagrangian} \\
    &+ \kappa_i \ . \ h_i(z_i) + (\nu/2) \norm{h_i(z_i)}^2 \nonumber\\
    &+ \eta_i \ . \ (z_i - \tilde{z}) + (\rho / 2) \norm{z_i - \tilde{z}}^2 \nonumber
\end{align}
where $\kappa_i \in \mathbb{R}^{m_i}$, $\eta_i \in \mathbb{R}^n$ are the dual variables corresponding to the equality constraints (\ref{eq:consensus_h_constraint}) and consensus constraint (\ref{eq:consensus_z_admm_constraint}) respectively. The constants $\nu$ and $\rho$ are positive real constants.
\end{definition} 

\begin{definition} 
The \textit{Distributed Augmented Lagrangian} algorithm consists of the iterating the following steps:
\begin{subequations} \label{eq:dec_algo}
\begin{align}  
{z^{k+1}_{i}} &:= \min_{z_i^k} L_{i, \nu, \rho}(\tilde{z}^k, z_i^k, \kappa_i^k, \eta_i^k) \label{eq:dec-algo-newton}\\
\kappa_i^{k+1} &:= \kappa_i^{k} + \nu h_i(z_i^{k+1}) \label{eq:dec-algo-dual-eq} \\
\tilde{z}^{k+1} &:= \frac{1}{N}\sum_i{z_i^{k+1}} \label{eq:dec-z_update} \\
\eta_i^{k+1} &:= \eta_i^{k} + \rho (z_i^{k+1} - \tilde{z}^{k+1}) \label{eq:dec-dual-admm}
\end{align}
\end{subequations}
\end{definition} 

At each iteration, the steps (\ref{eq:dec-algo-newton}) and (\ref{eq:dec-algo-dual-eq}) are applied for each of subproblem (for each $i \in [1, N]$). These sub-steps are parallelizable since they are fully independent from each other. On the other hand, the step (\ref{eq:dec-z_update}) is a centralized step averaging the results of the unconstrained minimizations (\ref{eq:dec-algo-newton}).

\subsection{Proof overview}
The proof proceeds in two steps:
\begin{itemize}
\item We first define the \textit{Constrained ADMM} algorithm, and show its convergence and optimality. This algorithm is closer to the ADMM standard form. It decomposes an optimization problem in only two subproblems, and performs the unconstrained minimization steps in sequence. It differs from the standard form, since one of the subproblems has an additional equality constraint.
\item Second, we show that the \textit{Distributed Augmented Lagrangian} can actually be rewritten as a special case of the \textit{Constrained ADMM}.
\end{itemize}
Taken together, those two steps prove convergence and optimality of the \textit{Distributed Augmented Lagrangian}. 

\subsection{Constrained ADMM algorithm} \label{constrained_admm}
Let $x \in \mathbb{R}^n$, $y \in \mathbb{R}^n$, $f:\mathbb{R}^{n} \rightarrow \mathbb{R}$ be a derivable cost function, $g:\mathbb{R}^{n} \rightarrow \mathbb{R}$ be a cost function proper, closed and convex, and $h:\mathbb{R}^{n} \rightarrow \mathbb{R}^m$ be a derivable equality constraints vector-valued function.
\begin{definition} We define the \textit{Constrained ADMM} optimization objective as:
\begin{subequations}
\begin{align}  
  \min_{x, y}&{
  \ f(x) + g(y)
  },\\
 &\text{s.t.} \notag \\
 & h(x) = 0, \label{eq:constrained_admm_eq_constraint} \\
 & x = y. \label{eq:constrained_admm_consensus_constraint}
\end{align}
\end{subequations}
\end{definition}

We note that this optimization objective is not symmetric:
\begin{itemize}
\item The equality constraints applies only on the $x$.
\item We require $f$ and $h$ to be derivable, whereas $g$ doesn't need to be derivable but we require it to be proper, closed and convex instead.
\end{itemize} 
The reason for this non-symmetry will become clearer in Section~\ref{sec:equivalence}. The functions $f$ and $h$ will represent the aggregation of the cost and constraint functions over the different subproblems. The function $g$ will be used as an indicator function taking values in $\{0, +\infty\}$ to enforce structure on $x$ and $y$.

\begin{definition} We define the \textit{Constrained ADMM} Augmented Lagrangian as:
\begin{align}  
  L_{\nu, \rho}(x, y, \kappa, \eta) &= 
  f(x) + g(y)\\
    &+ \kappa \ . \ h(x) + (\nu/2) \norm{h(x)}^2 \nonumber\\
    &+ \eta \ . \ (x - y) + (\rho / 2) \norm{x - y}^2 \nonumber,
\end{align}
where $\kappa \in \mathbb{R}^m$, $\eta \in \mathbb{R}^n$ are the dual variables corresponding to the equality constraint (\ref{eq:constrained_admm_eq_constraint}) and consensus constraint (\ref{eq:constrained_admm_consensus_constraint}) respectively. The constants $\nu$ and $\rho$ are positive real constants.
\end{definition}

\begin{definition} We define \textit{Constrained ADMM} algorithm as:
\begin{subequations}
\begin{align}  
  x^{k+1} &:= \min_{x} L_{\nu, \rho}(x, y^{k}, \eta^k)\\
  y^{k+1} &:= \min_{y} L_{\nu, \rho}(x^{k+1}, y, \eta^k)\\
  \kappa^{k+1} &:= \kappa^{k} + \nu h(x^{k+1})\\
  \eta^{k+1} &:= \eta^{k} + \rho(x^{k+1} - y^{k+1})
\end{align}
\end{subequations}
\end{definition}


\begin{theorem} \label{th:theorem_1}
If strong duality holds, meaning that there exists an optimal solution $x^{\star}$, $y^{\star}$ and lagrange multipliers $\kappa^{\star}$, and $\eta^{\star}$ such that $(x^{\star}, y^{\star}, \kappa^{\star}, \eta^{\star})$ is a saddle point of the Lagrangian $L_{0, 0}$, then the \textit{Constrained ADMM} algorithm converges to this optimum, $x^k \rightarrow x^{\star}$, $y^k \rightarrow y^{\star}$, $x^k \rightarrow x^{\star}$, $\kappa^k \rightarrow \kappa^{\star}$, $\eta^k \rightarrow \eta^{\star}$.
\end{theorem}

\subsection{Constrained ADMM convergence proof} \label{constrained_admm_proof}

We first introduce notation and three inequalities that will be used throughout the proof. We note $r^k$ the deviation between the two optimization variables:
\begin{subequations}
\begin{align}  
  r^k = x^k - y^k \nonumber
\end{align}
\end{subequations}
%\begin{remark}
%By definition $x^{\star} = y^{\star}$, therefore Theorem~\ref{th:theorem_1} implies that $r^k \rightarrow 0$ which means that the consensus constraint is satisfied.
%\end{remark}

We note $p^k$ the sum of the two costs functions:
%\begin{subequations}
\begin{equation}
  p^k = f(x^k) + g(y^k) \nonumber
\end{equation}
%\end{subequations}

\begin{definition} \label{def:vk} We define $V^k$ as a weighted sum of the squared distance from the optimum of the dual variables $\kappa$ and $\eta$ and the second primal variable $y$:
%\begin{subequations}
\begin{equation}  
  V^k = (1/\nu)\norm{\kappa^k-\kappa^{\star}}^2
+ (1/\rho)\norm{\eta^k-\eta^{\star}}^2
+ \rho \norm{y^k - y^{\star}}^2
\end{equation}
%\end{subequations}
\end{definition}

%\begin{remark}
The value of $V^k$ is not known during the algorithm execution since it depends on the unknown variables $x^{\star}, y^{\star}, \kappa^{\star}, \eta^{\star}$, but this value will be used to articulate the proof.
%\end{remark}

Finally, we introduce inequalities that hold throughout the algorithm.
Those inequalities will proven in Section~\ref{sec:inequalities_proof}.

\begin{definition}

We define two inequalities giving a lower and upper bound of the deviation from the optimum at the $k\textsuperscript{th}$ iteration:

Optimum deviation lower bound:
\begin{align} \label{eq:a_3}
p^{\star} - p^{k+1} \leq \kappa^{\star} \ .\ h(x^{k+1}) + \eta^{\star} \ . \ r^{k+1}  
\end{align}

Optimum deviation upper bound:
%\begin{subequations}
\begin{align}  \label{eq:a_2}
p^{k+1} - p^{\star} \leq - \kappa^{k+1} \ .\ h(x^{k+1}) - \eta^{k+1} \ .\ r^{k+1} + \rho (y^{k+1} - y^{k}) \ .\ (-r^{k+1} - (y^{k+1} - y^{\star})) 
\end{align}
%\end{subequations}
\end{definition}

\begin{definition}
We define the Value decay inequality as:
\begin{align}  \label{eq:a_1}
V^{k+1} - V^k\leq - \nu \norm{h(x^{k+1})}^2 - \rho \norm{r^{k+1}}^2 - \rho \norm{y^{k+1} - y^k}^2
\end{align}
\end{definition}

\subsubsection{Convergence proof when assuming the equalities (\ref{eq:a_3}), (\ref{eq:a_2}) and (\ref{eq:a_1}) to be true}

\begin{theorem} \label{th:theorem_2}
If the three inequalities (\ref{eq:a_3}), (\ref{eq:a_2}) and (\ref{eq:a_1}) are true, then the \textit{Constrained ADMM} algorithm converges to the optimal values $x^{\star}$, $y^{\star}$, $\kappa^{\star}$ and $\eta^{\star}$.
\end{theorem}

\begin{proof}[Proof of Convergence]
%\paragraph{Convergence}
%aaa

Summing the (inequality~\ref{eq:a_1}) for an infinite number of iterations gives the following inequality:
\begin{equation*}
V^{\infty} - V^0 \leq - \nu \sum_{k=0}^{\infty}{\norm{h(x^{k+1})}^2} - \rho \sum_{k=0}^{\infty}{\norm{r^{k+1}}^2 + \norm{y^{k+1} - y^{k}}^2}, \label{eq:residual_sum_1}
\end{equation*}
which can be rewritten as,
\begin{align}  
\nu \sum_{k=0}^{\infty}{\norm{h(x^{k+1})}^2} + \rho \sum_{k=0}^{\infty}{\norm{r^{k+1}}^2 + \norm{y^{k+1} - y^{k}}^2} \leq V^0 - V^{\infty}. \label{eq:residual_sum_2}
\end{align}

%\Rightarrow 

By definition, $V^k$ is always a positive, since it is the sum of the norm of vectors weighed by positive numbers. In addition, the Value decay inequality (\ref{eq:a_1}) implies that $V^k \leq V^0$. Therefore $V^0 - V^{\infty}$ is finite and positive.

The left side of the inequality~(\ref{eq:residual_sum_2}) is the sum of an infinity of positive terms. This sum is bounded by $V^0 - V^{\infty}$ which implies that the summed elements tend to zero, i.e. $h(x^{k+1}) \rightarrow 0 $, $r^k \rightarrow 0$ and $y^{k+1} - y^{k} \rightarrow 0$ when $k \rightarrow \infty$.
This respectively means that the equality constraint~(\ref{eq:constrained_admm_eq_constraint}) is enforced, that the two local variables $x$ and $y$ reach a consensus~(\ref{eq:consensus_z_admm_constraint}), and that the algorithm becomes stationary.
\end{proof}

\begin{proof}[Proof of Optimality]
Inequality~(\ref{eq:a_3}) gives an lower-bound of $p^{k+1} - p^{\star}$. We showed in the convergence proof, that $h(x^{k+1}) \rightarrow 0$ and $r^{k+1} \rightarrow 0$. It therefore implies that the lower bound tends to zero. %\textcolor{blue}{How can we be sure that $\eta^{\star}$ and $\kappa^{\star}$ are not infinite?}


Inequality~(\ref{eq:a_2}) gives an upper-bound of $p^{k+1} - p^{\star}$. We showed earlier that $h(x^{k+1}) \rightarrow 0$,  $r^{k+1} \rightarrow 0$ and $y^{k+1} - y^{k} \rightarrow 0$. In addition, the fact that $0 \leq V^k \leq V^0$ implies that $\kappa^{k+1}$, $\eta^{k+1}$, and $y^{k+1} - y^{\star}$ are bounded. The upper bound is therefore a sum of three terms which are each a multiplication between a finite term and a quantity tending to zero. The upper-bound therefore tends to zero.
% \textcolor{blue}{Same question here? KKT conditions imply bounded?}

Since both the upper and lower bounds of $p^{k+1} - p^{\star}$ tend to zero, it implies that $p^k \rightarrow p^{\star}$ which is the objective convergence.
\end{proof}


\subsubsection{Proof of the inequality (\ref{eq:a_3})} \label{sec:inequalities_proof}

\begin{theorem}[Optimum deviation lower-bound] If there exists an optimal solution $x^{\star}$, $y^{\star}$ and lagrange multipliers $\kappa^{\star}$, and $\eta^{\star}$ such that $(x^{\star}, y^{\star}, \kappa^{\star}, \eta^{\star})$ is a saddle point of the Lagrangian $L_{0, 0}$ then the inequality~(\ref{eq:a_3}) is true, i.e.
\begin{align*}
p^{\star} - p^{k+1} \leq \kappa^{\star} \ .\ h(x^{k+1}) + \eta^{\star} \ . \ r^{k+1}  
\end{align*}
\end{theorem}

\begin{proof}
Since $(x^{\star}, y^{\star}, \kappa^{\star}, \eta^{\star})$ is a saddle point of $L_{0, 0}$, we have
% \textcolor{blue}{Is saddle point enough here?}s
\begin{align*}  
L_{0, 0}(x^{\star}, y^{\star}, \kappa^{\star}, \eta^{\star}) &\leq L_{0, 0}(x^{k+1}, y^{k+1}, \kappa^{\star}, \eta^{\star})
\end{align*}
By definition, $h(x^{\star}) = 0$, $x^{\star} = y^{\star}$, and $\rho = \nu = 0$ such that the Lagrangian on the left side reduces to the cost terms $f(x^{\star}) + g(x^{\star})$. On the right side the Lagrangian is composed to the cost term $f(x^{k+1}) + g(x^{k+1})$ and of the lagrange terms for the equality and consensus constraints, such that it gives,
\begin{align*}  
f(x^{\star}) + g(x^{\star}) &\leq f(x^{k+1}) + g(x^{k+1}) + \kappa^{\star}\ .\ h(x^{k+1}) + \eta^{\star}\ .\ (x^{k+1} - y^{k+1})
\end{align*}
which is Inequality~(\ref{eq:a_3}) when replacing $f(x) + g(y)$ by $p$ and $x-y$ by $r$ according to their definitions:
\begin{align*}  
p^{\star} - p^{k+1} &\leq \kappa^{\star} \ .\ h(z_0^{k+1}) + \eta^{\star} \ .\ r^{k+1}.
\end{align*}
\end{proof}

\subsubsection{Proof of the inequality (\ref{eq:a_2})}
\begin{theorem}[Optimum deviation upper-bound]
 If there exists an optimal solution $x^{\star}$, $y^{\star}$ and lagrange multipliers $\kappa^{\star}$, and $\eta^{\star}$ such that $(x^{\star}, y^{\star}, \kappa^{\star}, \eta^{\star})$ is a saddle point of the Lagrangian $L_{0, 0}$ then the inequality~(\ref{eq:a_2}) is true, i.e.
\begin{align*}
p^{k+1} - p^{\star} \leq - \kappa^{k+1} \ .\ h(x^{k+1}) - \eta^{k+1} \ .\ r^{k+1} + \rho (y^{k+1} - y^{k}) \ .\ (-r^{k+1} - (y^{k+1} - y^{\star}))
\end{align*} 
\end{theorem}

\begin{proof}
\item
\paragraph{Using optimality conditions w.r.t the first optimization variable:}
By definition, $x^{k+1}$ minimizes $L_{\nu, \rho}(\Z, y^k, \kappa^k, \eta^{k})$. Since  $f$ and $h$ are differentiable, the Lagrangian is differentiable and a necessary optimality condition is that the gradient is zero in $x^{k+1}$, i.e.
%\paragraph{First part using $z_0$:}
%\begin{subequations}
%\begin{align} 
%\frac{\partial L_{\nu, \rho} (x^{k+1}, y^k, \kappa^k, %\eta^k) = 0 \nonumber \\ 
%\frac{\partial f}{\partial x} (x^{k+1}) + \kappa^k \cdot \frac{\partial h}{\partial x} (x^{k+1}) + \nu \ h(x^{k+1}) \cdot \frac{\partial h}%\end{align}
%\end{subequations}
\begin{subequations}
\begin{gather} 
\nabla_x L_{\nu, \rho} (x^{k+1}, y^k, \kappa^k, \eta^k) = 0, \nonumber \\ 
\nabla f (x^{k+1}) + \kappa^k \cdot \mathbb{J}_h (x^{k+1}) + \nu h(x^{k+1}) \cdot \mathbb{J}_h(x^{k+1}) + \eta^k + \rho (x^{k+1} - y^{k}) = 0. \nonumber
\end{gather}
\end{subequations}

We develop further the second term using $\kappa^{k} = \kappa^{k+1} - \nu h(x^{k+1})$, which has for effect to cancel the third term. Similarly, we use $\eta^{k} = \eta^{k+1} - \rho (x^{k+1} - y^{k+1})$ for the third term, which can then be combined with the fourth term and gives
%\begin{subequations}
%\begin{align} 
%\nabla f(x^{k+1}) +
% (\kappa^{k+1} - \nu h(x^{k+1})) \cdot \mathbb{J}_h (x^{k+1}) + \nu h(x^{k+1}) \cdot \mathbb{J}(x^{k+1}) +
% \eta^{k+1} - \rho (z_0^{k+1} - z_1^{k+1}) + \rho (z_0^{k+1} - z_1^{k}) = 0 \nonumber \\
%\frac{\partial}{\partial z_0} c_0(z_0^{k+1}) + \kappa^{k+1} %\frac{\partial h}{\partial z_0} (z_0^{k+1})  + \eta^{k+1} + \rho ( z_1^{k+1} - z_1^{k}) = 0 \nonumber
%\end{align}
%\end{subequations}
\begin{subequations}
\begin{align} 
\nabla f(x^{k+1}) +
 \kappa^{k+1} \cdot \mathbb{J}_h (x^{k+1}) +
 \eta^{k+1} + \rho ( y^{k+1} - y^{k}) = 0 \nonumber
\end{align}
\end{subequations}

This implies, that $x^{k+1}$ minimizes
%\begin{subequations}
\begin{align*} 
f(x) + \kappa^{k+1} \cdot h(x) + (\eta^{k+1} + \rho (y^{k+1} - y^{k})) \cdot x
\end{align*}
%\end{subequations}

It follows that its evaluation at $x^{k+1}$ is lower than at $x^{\star}$ which gives the following inequality
%\begin{subequations}
\begin{align} \label{eq:proof_A_2_first_term}
f(x^{k+1}) + \kappa^{k+1}h(x^{k+1}) + (\eta^{k+1} + \rho (y^{k+1} - y^{k})) \cdot x^{k+1} \leq  f(x^{\star}) + (\eta^{k+1} + \rho (y^{k+1} - y^{k})) \cdot y^{\star}
\end{align}
Note: In the expression above, we use the fact that $h(x^{\star}) = 0$, by definition.

\paragraph{Optimality conditions w.r.t the second optimization variable:}
By definition, $y^{k+1}$ minimizes $L_{\nu, \rho}(x^{k+1},\ \Z \ , \kappa^k, \eta_{k})$. Since $g$ is closed, proper and convex, the Lagrangian is subdifferentiable, and a necessary and sufficient optimality condition is therefore that 0 belongs to the subderivatives of the Langrangian in $y^{k+1}$:
% (\textcolor{blue}{Should we here be more precise and argument that by the virtual of the update rule, $\chi(z_1^{k}) = 0$, which in turn removes the term $c_1$? -> No because it doesn't work as easily, here the variable is $z_1$ not the $\bar{z}_1$}).
%\begin{subequations}
\begin{align*} 
0 \in \partial_y L_{\nu, \rho}(x^{k+1}, y^{k+1}, \kappa^k, \eta^k)  \nonumber
\end{align*}
The derivation of the lagrange term as well as the square penalty with respect to $y$ are trivial, such that the subdifferential notation remains only on $g$ giving:
\begin{align*} 
0 \in \partial g(y^{k+1}) - \eta^k - \rho (x^{k+1} - y^{k+1}) \nonumber 
\end{align*}
%\end{subequations}
We now use $\eta^{k} = \eta^{k+1} - \rho (x^{k+1} - y^{k+1})$ for the second term, which cancels the third term and gives:
\begin{align*} 
0 \in \frac{\partial}{\partial z_1} c_1(z_1^{k+1}) - \eta^{k+1}
\end{align*}

This implies that $y^{k+1}$ minimizes
\begin{align} 
g(y) - \eta^{k+1} \cdot y \label{eq:g_intermediary}
\end{align}

Comparing the evaluations in $y^{k+1}$ and $y^{\star}$ leads to the following inequality:
\begin{align} \label{eq:proof_A_2_second_term}
g(y^{k+1}) - \eta^{k+1} \cdot \ y^{k+1} \leq g(y^{\star}) - \eta^{k+1} \cdot \ y^{\star}
\end{align}

\paragraph{Summing the two inequalities:}
Summing up (\ref{eq:proof_A_2_first_term}) and (\ref{eq:proof_A_2_second_term}) gives:
\begin{subequations}
\begin{align}
f(x^{k+1}) + \kappa^{k+1} \cdot h(x^{k+1}) + (\eta^{k+1} + \rho (y^{k+1} - y^{k})) \cdot x^{k+1} \nonumber \\ +\ g(y^{k+1}) - \eta^{k+1} \cdot y^{k+1} \nonumber \\ \leq \nonumber \\ f(x^{\star}) + (\eta^{k+1} + \rho (y^{k+1} - y^{k})) \cdot x^{\star} \nonumber\\+\ g(y^{\star}) - \eta^{k+1}\ . \ y^{\star} \nonumber
\end{align}
\end{subequations}
We now separate the cost terms with $f$ and $g$ (moved to the left side) from the other terms which are moved to the right side. Using the notation with $p$, this gives:
\begin{align*}
p^{k+1} - p^{\star} \\
 \leq \\ - \kappa^{k+1} \cdot h(x^{k+1}) - (\eta^{k+1} + \rho (y^{k+1} - y^{k})) \cdot x^{k+1} \\ + (\eta^{k+1} + \rho (y^{k+1} - y^{k})) \cdot x^{\star} + \eta^{k+1} \cdot y^{k+1} - \eta^{k+1} \cdot y^{\star}
\end{align*}

We now use the fact that $x^{\star} = y^{\star}$ which eliminates the terms with $\eta^{k+1} \cdot z_1^{k+1}$ and gives:
\begin{align*}
p^{k+1} - p^{\star}
 &\leq - \kappa^{k+1} \cdot h(x^{k+1}) - (\eta^{k+1} + \rho (y^{k+1} - y^{k})) \cdot x^{k+1} + \rho (y^{k+1} - y^{k}) \cdot y^{\star} + \eta^{k+1} \cdot y^{k+1} \\
\intertext{Regrouping the terms around and using the notation $r^{k+1} = x^{k+1} - y^{k+1}$ leads to:}
p^{k+1} - p^{\star}
 &\leq - \kappa^{k+1} \cdot h(x^{k+1}) - \eta^{k+1} \cdot r^{k+1} - \rho (y^{k+1} - y^{k}) \cdot x^{k+1} + \rho (y^{k+1} - y^{k}) \cdot y^{\star}  \\
\intertext{We now factorize the last terms around $\rho (y^{k+1} - y^{k})$ to get:}
p^{k+1} - p^{\star}
 &\leq - \kappa^{k+1} \cdot h(x^{k+1}) - \eta^{k+1} \cdot r^{k+1} + \rho (y^{k+1} - y^{k}) \cdot (-x^{k+1} + y^{\star}) \\
\intertext{The last term $-x^{k+1} + y^{\star}$ can be trivially rewritten into $-x^{k+1} + y^{k+1} - y^{k+1} + y^{\star}$, which is $-r^k - (y^{k+1} - y^{\star})$, which results in}
 p^{k+1} - p^{\star}
 &\leq - \kappa^{k+1} \cdot h(x^{k+1}) - \eta^{k+1}\ .\ r^{k+1} + \rho (y^{k+1} - y^{k}) . (-r^{k+1} - (y^{k+1} - y^{\star})),
\end{align*}
which is the inequality (\ref{eq:a_2}).
\end{proof}

\subsubsection{Proof of the inequality (\ref{eq:a_1})}
\begin{theorem}[Value decay]
 If there exists an optimal solution $x^{\star}$, $y^{\star}$ and lagrange multipliers $\kappa^{\star}$, and $\eta^{\star}$ such that $(x^{\star}, y^{\star}, \kappa^{\star}, \eta^{\star})$ is a saddle point of the Lagrangian $L_{0, 0}$ then the inequality~(\ref{eq:a_1}) is true, i.e.
\begin{align*}
V^{k+1} - V^k \leq - \nu \norm{h(x^{k+1})}^2 - \rho \norm{r^{k+1}}^2 -\rho \norm{y^{k+1} - y^k}^2.
\end{align*} 
\end{theorem}

\begin{proof}
%\paragraph{Proof of A.1} \label{sec:a_1}
Adding the inequalities (\ref{eq:a_3}) and (\ref{eq:a_2}) gives:
\begin{align}
&0 \leq -\kappa^{k+1} \cdot h(x^{k+1}) - \eta^{k+1} \cdot r^{k+1} + \rho (y^{k+1} - y^{k}) \cdot (-r^{k+1} - (y^{k+1} - y^{\star})) + \kappa^{\star} \cdot h(x^{k+1}) + \eta^{\star} \cdot r^{k+1} \nonumber \\
\intertext{Flipping the inequality and factorizing the terms involving $h(x^{k+1})$ leads to:}
&(\kappa^{k+1} - \kappa^{\star}) \cdot h(x^{k+1}) + \eta^{k+1} \cdot r^{k+1} - \rho (y^{k+1} - y^{k}) \cdot (-r^{k+1} - (y^{k+1} - y^{\star})) - \eta^{\star} \cdot r^{k+1} \leq 0 \nonumber \\
\intertext{We now regroup the terms with $\eta$ to get:}
&(\kappa^{k+1} - \kappa^{\star}) \cdot h(x^{k+1}) + (\eta^{k+1} - \eta^{\star}) \cdot r^{k+1} - \rho (y^{k+1} - y^{k}) \cdot (-r^{k+1} - (y^{k+1} - y^{\star})) \leq 0 \nonumber \\
\intertext{We now simply multiply by 2 to obtain:}
&2(\kappa^{k+1} - \kappa^{\star}) \cdot h(x^{k+1}) + 2(\eta^{k+1} - \eta^{\star}) \cdot r^{k+1} - 2\rho (y^{k+1} - y^{k}) \cdot (-r^{k+1} - (y^{k+1} - y^{\star})) \leq 0 \label{eq:a2_plus_a3_to_rewrite}
\end{align}

This inequality is composed of three terms that we will rewrite one by one in the next sections. The main goal is to make appear the terms $\norm{\kappa^{k} - \kappa^{\star}}^2$, $\norm{\eta^{k} - \eta^{\star}}^2$, $\norm{y^{k} - \eta^{\star}}^2$ which are the compounds of $V^k$.

\paragraph{Rewriting the first term of inequality (\ref{eq:a2_plus_a3_to_rewrite})} \label{sec:rewrite_first_term}
The term to rewrite is
\begin{align*}
2 (\kappa^{k+1} - \kappa^{\star}) \cdot h(x^{k+1}).
\end{align*}
We use the fact that $\kappa^{k+1} = \kappa^{k} + \nu h(x^{k+1})$ which gives
\begin{align*}
2 (\kappa^{k} + \nu h(z^{k+1}) - \kappa^{\star}) \cdot h(x^{k+1})
\end{align*}
Developing and splitting the term involving $h(x^{k+1})$ into two identical parts gives:
\begin{align*}
2 (\kappa^{k} - \kappa^{\star}) .\ h(x^{k+1}) + \nu \norm{h(x^{k+1})}^2 + \nu \norm{h(x^{k+1})}^2
\end{align*}
Substituing $h(x^{k+1}) = \frac{1}{\nu}(\kappa^{k+1} - \kappa^{k})$ in the first two terms gives
\begin{align*}
\frac{2}{\nu}(\kappa^{k} - \kappa^{\star}) \cdot (\kappa^{k+1} - \kappa^{k}) + \frac{1}{\nu} \norm{\kappa^{k+1} - \kappa^{k}}^2 + \nu \norm{h(x^{k+1})}^2
\end{align*}
We rewrite further the first term using $\kappa^{k+1} - \kappa^{k} = (\kappa^{k+1} - \kappa^{\star}) + (\kappa^{\star} - \kappa^{k})$ to expand the first term
\begin{align*}
\frac{2}{\nu}(\kappa^{k} - \kappa^{\star}) \cdot ((\kappa^{k+1} - \kappa^{\star}) + (\kappa^{\star} - \kappa^{k})) + \frac{1}{\nu} \norm{\kappa^{k+1} - \kappa^{k}}^2 + \nu \norm{h(x^{k+1})}^2
\intertext{Developing the first term leads to:}
-\frac{2}{\nu}\norm{\kappa^{k} - \kappa^{\star}}^2 + \frac{2}{\nu} (\kappa^{k} - \kappa^{\star}) \cdot (\kappa^{k+1} - \kappa^{\star}) + \frac{1}{\nu} \norm{\kappa^{k+1} - \kappa^{k}}^2 + \nu \norm{h(x^{k+1})}^2
\end{align*}

We now rewrite the third term using $\kappa^{k+1} - \kappa^{k} = (\kappa^{k+1} - \kappa^{\star}) + (\kappa^{\star} - \kappa^{k})$ again:
\begin{align*}
-\frac{2}{\nu}\norm{\kappa^{k} - \kappa^{\star}}^2 + \frac{2}{\nu} (\kappa^{k} - \kappa^{\star}) \cdot (\kappa^{k+1} - \kappa^{\star}) + \frac{1}{\nu} \norm{(\kappa^{k+1} - \kappa^{\star}) + (\kappa^{\star} - \kappa^{k})}^2 + \nu \norm{h(x^{k+1})}^2
\end{align*}
Developping the norm gives:
\begin{align*}
-\frac{2}{\nu}\norm{\kappa^{k} - \kappa^{\star}}^2 + \frac{2}{\nu} (\kappa^{k} - \kappa^{\star}) \cdot & (\kappa^{k+1} - \kappa^{\star}) + \frac{1}{\nu} \norm{\kappa^{k+1} - \kappa^{\star}}^2\\& + \frac{1}{\nu}\norm{\kappa^{\star} - \kappa^{k}}^2 + \frac{2}{\nu}(\kappa^{k+1} - \kappa^{\star}) \cdot (\kappa^{\star} - \kappa^{k}) + \nu \norm{h(x^{k+1})}^2
\end{align*}
The terms $\frac{2}{\nu} (\kappa^{k} - \kappa^{\star}) \cdot (\kappa^{k+1} - \kappa^{\star})$ cancel themselves and the terms with $\norm{\kappa^{k} - \kappa^{\star}}^2$ can be regrouped, giving:
\begin{align}
(1 / \nu) \left( \norm{\kappa^{k+1} - \kappa^{\star}}^2 - \norm{\kappa^{\star} - \kappa^{k}}^2 \right) + \nu \norm{h(x^{k+1})}^2
\end{align}

\paragraph{Rewriting the second term}
The term to rewrite is  
\begin{align*}
2 (\eta^{k+1} - \eta^{\star}) \ .\ r^{k+1}
\end{align*}
This is the exact equivalent of the first term rewritten in Section~\ref{sec:rewrite_first_term} with $\eta^{k+1}$, $\eta^{\star}$ and $r^{k+1}$ instead of $\kappa^{k+1}$, $\kappa^{\star}$ and $h(x^{k+1})$.

Therefore a similar argument, (using the fact that $\eta^{k+1} = \eta^{k} + \rho r^{k+1}$) leads to:
\begin{align}
(1 / \rho) \left( \norm{\eta^{k+1} - \eta^{\star}}^2 - \norm{\eta^{\star} - \eta^{k}}^2 \right) + \rho \norm{r^{k+1}}^2 \label{eq:rewritten_second_term}
\end{align} 

\paragraph{Rewriting the third term of inequality (\ref{eq:a2_plus_a3_to_rewrite})}

We now rewrite the third term (\ref{eq:a2_plus_a3_to_rewrite}) to which we add the term $\rho \norm{r^{k+1}}^2$ coming from the rewritten second term (\ref{eq:rewritten_second_term}). The term to rewrite is therefore:
\begin{align*}
\rho \norm{r^{k+1}}^2 + 2 \rho (y^{k+1} - y^{k}) \cdot r^{k+1} + 2 \rho (y^{k+1} - y^{k})\ .\ (y^{k+1} - y^{\star})
\end{align*}

We use $y^{k+1} - y^{\star} = (y^{k+1} - y^{k}) + (y^k - y^{\star})$ in the last term and develop it to obtain:
\begin{align*}
\rho \norm{r^{k+1}}^2 + 2 \rho (y^{k+1} - y^{k}) \cdot r^{k+1} + 2 \rho \norm{y^{k+1} - y^{k}}^2 + 2 \rho (y^{k+1} - y^{k}) \cdot ((y^k - y^{\star}))
\end{align*}
Observing that $\rho \norm{r^{k+1}}^2 + 2 \rho (y^{k+1} - y^{k}) \cdot r^{k+1} = \rho \norm{r^{k+1} + (y^{k+1} - y^k)}^2 - \rho \norm{y^{k+1} - y^{k}}^2$, we rewrite the first two terms and combine it with the third term to get:
\begin{align*}
\rho \norm{r^{k+1} + (y^{k+1} - y^k)}^2 + \rho \norm{y^{k+1} - y^{k}}^2 + 2 \rho (y^{k+1} - y^{k}) \cdot ((y^k - y^{\star}))
\end{align*}
We now rewrite the last two terms using $y^{k+1} - y^k = (y^{k+1} - y^{\star}) - (y^{k} - y^{\star})$,
\begin{align*}
\rho \norm{r^{k+1} + (y^{k+1} - y^k)}^2 + \rho \norm{(y^{k+1} - y^{\star}) - (y^{k} - y^{\star})}^2 + 2 \rho ((y^{k+1} - y^{\star}) - (y^{k} - y^{\star})) \cdot (y^k - y^{\star})
\end{align*}
and develop further which gives:
\begin{align*}
\rho \norm{r^{k+1} + (y^{k+1} - y^k)}^2 + \rho \norm{y^{k+1} - y^{\star}}^2 + \rho \norm{ y^{k} - y^{\star}}^2 - 2\rho (y^{k+1} - y^{\star}) \cdot (y^{k} - y^{\star}) \\+ 2 \rho ((y^{k+1} - y^{\star}) - (y^{k} - y^{\star})) \cdot ((y^k - y^{\star}))
\end{align*}
The terms starting with $2\rho$ partially cancel themselves resulting in the following,
\begin{align*}
\rho \norm{r^{k+1} + (y^{k+1} - y^k)}^2 + \rho \norm{(y^{k+1} - y^{\star})}^2 + \rho \norm{ y^{k} - y^{\star}}^2 - 2 \rho \norm{y^k - y^{\star}}^2
\end{align*}
and finally,
\begin{align}
\rho \norm{r^{k+1} + (y^{k+1} - y^k)}^2 + \rho \left( \norm{(y^{k+1} - y^{\star})}^2 -  \norm{y^k - y^{\star}}^2 \right).
\end{align}

\paragraph{Bringing the rewritten terms back together}
Adding the first, second and third terms and bringing back the inequality gives:
\begin{align*}
\frac{1}{\nu} \left( \norm{\kappa^{k+1} - \kappa^{\star}}^2 - \norm{\kappa^{\star} - \kappa^{k}}^2 \right) & + \nu \norm{h(x^{k+1})}^2 \\ &+\frac{1}{\rho} \left( \norm{\eta^{k+1} - \eta^{\star}}^2 - \norm{\eta^{\star} - \eta^{k}}^2 \right) \\ &+ \rho \norm{r^{k+1} + (y^{k+1} - y^k)}^2 + \rho \left( \norm{(y^{k+1} - y^{\star})}^2 -  \norm{y^k - y^{\star}}^2 \right) \leq 0
\end{align*}
The terms in large parenthese are exactly the compounds of $V^{k+1} - V^k$ such that one can rewrite the expression into:
\begin{align*}
V^{k+1} - V^k + \nu \norm{h(x^{k+1})}^2 + \rho \norm{r^{k+1} + (y^{k+1} - y^k)}^2 \leq 0
\end{align*}
and equivalently,
\begin{align*}
V^{k+1} - V^k \leq -\nu \norm{h(x^{k+1})}^2 - \rho \norm{r^{k+1} + (y^{k+1} - y^k)}^2
\end{align*}
which gives the following expression when developing the last term
\begin{align} 
V^{k+1} - V^k \leq - \nu \norm{h(x^{k+1})}^2 - \rho \norm{r^{k+1}}^2 -\rho \norm{y^{k+1} - y^k}^2 - 2\rho r^{k+1} \cdot (y^{k+1} - y^k). \label{eq:almost_a_1} 
\end{align}
This is almost the inequality~(\ref{eq:a_1}), except for the last term $2\rho r^{k+1} \cdot (y^{k+1} - y^k)$ which is not present in~(\ref{eq:a_1}). To show (\ref{eq:a_1}) it is therefore sufficient to  that $\rho r^{k+1} \cdot (y^{k+1} - y^k) \geq 0$.

To show this, we use the fact that $y^{k+1}$ minimizes $g(y) - \eta^{k+1} \cdot y$ and that $y^{k}$ minimizes $g(y) - \eta^{k} \cdot  y$ as it has been established in (\ref{eq:g_intermediary}). One can therefore write the two following inequalities:
\begin{align*}
g(y^{k+1}) - \eta^{k+1} \cdot y^{k+1} &\leq g(y^{k}) - \eta^{k+1} \cdot y^{k}\\
g(y^{k}) - \eta^{k} \cdot y^{k} &\leq g(y^{k+1}) - \eta^{k} \cdot y^{k+1}
\end{align*}

When summing these two inequalities, the cost terms involving $g$ cancel themselves such that it gives:

\begin{align*}
- \eta^{k+1}\ . \ z_1^{k+1} - \eta^{k}\ . \ z_1^{k} &\leq - \eta^{k+1}\ . \ z_1^{k} - \eta^{k}\ . \ z_1^{k+1}
\end{align*}
wich is equivalent to,
\begin{align*}
(\eta^{k+1} - \eta^{k}) \ . \ (z_1^{k+1} - z_1^{k}) \geq 0.
\end{align*}

Given the fact that $\eta^{k+1} - \eta^k = \rho r^{k+1}$, it implies that $\rho r^{k+1} \cdot (y^{k+1} - y^k) \geq 0$, which combined with (\ref{eq:almost_a_1}) therefore implies:

\begin{align} 
V^{k+1} - V^k \leq - \nu \norm{h(x^{k+1})}^2 - \rho \norm{r^{k+1}}^2 -\rho \norm{y^{k+1} - y^k}^2.
\end{align}
which is (\ref{eq:a_1}).

\end{proof}

\subsection{Distributed Augmented Lagrangian as a special case of Sequential Constrained ADMM} \label{sec:equivalence}

We will now show that that the \textit{Distributed Augmented Lagrangian} algorithm is in fact a particular case of \textit{Constrained ADMM} algorithm. 

Let $c_i: \mathbb{R}^n \rightarrow \mathbb{R}$ and $h_i: \mathbb{R}^{n} \rightarrow \mathbb{R}^m$ be $N$ derivable functions defining a \textit{Distributed Augmented Lagragian} problem.
\begin{align}  
  \min_{z_i}&{
  \ \sum_i{c_i(z_i)} \label{eq:equivalent_distributed}
  },\\
 &\text{s.t.} \notag \nonumber \\
 & h_i(z_i) = 0 ,\nonumber\\
 & z_i = \tilde{z}.\nonumber
\end{align}

We now introduce the optimization variable $z \in \mathbb{R}^{n \times N}$, stacking the sub-optimization variables $z_i$ i.e. $z = (z_0, .., z_{N-1})$.

Let now define $c:\mathbb{R}^{n \times N} \rightarrow \mathbb{R}$ as a function summing the $c_i$ costs, i.e.~$f(z) = \sum_i c_i(z_i)$.

Let $h:\mathbb{R}^{n \times N} \rightarrow \mathbb{R}^{m \times N}$ be an equality constraint function aggregating the constraints $h_i$, meaning that $h(z) = (h_0(z_0), ..., h_{N-1}(z_{N-1}))$.

Let $\chi$ the characteristic function of the subset of $\mathbb{R}^{n \times N}$ where $z$ is an aggregation of $N$~times the same value, i.e.  $\chi(z) = \chi(z_0, ..., z_{N-1}) = \begin{cases}
  0, & \text{if } z_0 = z_1 = .. = z_{N-1}, \\
  + \infty, &\text{otherwise}.
\end{cases}$.

The pre-requisites for applying the \textit{Constrained ADMM} algorithm are fulfilled: $c$ and $h$ are derivable, since the $c_i$ and $h_i$ are. In addition, it can be shown easily that $\chi$ is closed, proper and convex (convexity and properness are trivial, closeness comes from the fact the underlying set ${\{(z_0, ..., z_N) \in \mathbb{R}^{n \times N} \mid z_0 = ... = z_N}\}$ is itself closed).

One can therefore apply the \textit{Consensus ADMM} algorithm to the following problem:
\begin{align}  
  \min_{z, y}&{ 
  \ c(z) + \chi(y) \label{eq:equivalent_sequential}
  },\\
 &\text{s.t.} \notag \\
 & h(z) = 0 \nonumber \\
 & z = y, \nonumber \\
\end{align} 
which we will show is exactly the \textit{Distributed Augmented Lagrangian} algorithm.

We first establish that $\chi(y^k) = 0$ at all times during \textit{Constrained ADMM} algorithm execution, the equivalence of the two algorithm will follow as a consequence.

\begin{theorem} \label{th:theorem_chi_zero}
When applying the \textit{Constrained ADMM} algorithm on the \textit{Distributed Augmented Lagrangian} problem  (\ref{eq:equivalent_distributed}), the following statement is true:
\begin{align*}
\chi(y^k) = 0,\ \forall k \geq 1.
\end{align*}
\end{theorem}

\begin{proof}
By definition of the algorithm, we have $y^{k+1} = \min_{y} L_{\nu, \rho}(z^{k+1}, y, \kappa^k, \eta^k)$, with the Lagrangian being $L_{\nu, \rho}(z, y, \kappa, \eta) = 
  f(z) + \chi(y) + \kappa \cdot h(z) + \frac{\nu}{2} \norm{h(z)}^2 + \eta \cdot (x - y) + \frac{\rho}{2} \norm{x - y}^2$. One can prove easily by contradiction that minimizing the Lagrangian implies that $\chi(y^{k+1}) = 0$:
  
If there exist $y^{\star}$ minimizing the Lagrangian, with $\chi(y^{\star}) \neq 0$, then it follows from the definition of $\chi$ that $\chi(y^{\star}) = +\infty$, since the function $\chi$ takes only values in $\{0, +\infty\}$. We therefore have $L_{\nu, \rho}(z^{k+1}, y^{\star}, \kappa^k, \eta^k) = +\infty$ since the other terms of the Lagrangian have finite values. One can therefore construct a variable $y^{\star}_2$ which  is the $N$-fold concatenation of the $m$ first vector elements of $y^{\star}$, $y_2^{\star} = (y^{\star}, ..., y^{\star})$. By definition of $\chi$ and $y^{\star}_2$, we have $\chi(y_2^{\star}) = 0$, which implies that $L_{\nu, \rho}(z^{k+1}, y^{\star}_2, \kappa^k, \eta^k) < +\infty$. In other words, $L_{\nu, \rho}(z^{k+1}, y^{\star}_2, \kappa^k, \eta^k) < L_{\nu, \rho}(z^{k+1}, y^{\star}, \kappa^k, \eta^k)$ which contradicts the definition~of~$y^{\star}$.
\end{proof}

Since $\chi(y^k) = 0$, it means that we can define the $y$ fully by its first $m$ elements, meaning that we can introduce the variable $\tilde{z} \in \mathbb{R}^n$ such that $y = (\tilde{z}, ..., \tilde{z})$. 

With this notation in place, the correspondance between the two algorithms can be established:

\begin{theorem} \label{th:theorem_eq}
Applying the \textit{Constrained ADMM} algorithm on the problem (\ref{eq:equivalent_sequential}) is equivalent to applying the algorithm steps of the \textit{Distributed Augmented Lagrangian} algorithm on (\ref{eq:equivalent_distributed}), i.e.
\begin{alignat}{2}
&z^{k+1} := \min_{z} L_{\nu, \rho}(z, y^{k}, \kappa^k, \eta^k) \ \ &&\Longleftrightarrow\ \  {z^{k+1}_{i}} := \min_{z_i} L_{i, \nu, \rho}(z_i, \tilde{z}^k, \kappa_i^k, \eta_i^k) \label{th:eq_lagrangian_minimization} \\
&y^{k+1} := \min_{y} L_{\nu, \rho}(z^{k+1}, y, \kappa^k, \eta^k)\ \ &&\Longleftrightarrow\ \  \tilde{z}^{k+1} := \frac{1}{N}\sum_i{z_i^{k+1}} \label{th:eq_y_update} \\
&\kappa^{k+1} := \kappa^{k} + \nu h(z^{k+1})\ \  &&\Longleftrightarrow\ \  \kappa_i^{k+1} := \kappa_i^{k} + \nu h_i(z_i^{k+1}) \label{th:eq_kappa_update}\\
&\eta^{k+1} := \eta^{k} + \rho(z^{k+1} - y^{k+1})\ \  &&\Longleftrightarrow\ \  \eta_i^{k+1} := \eta_i^{k} + \rho (z_i^{k+1} - \tilde{z}^{k+1}) \label{th:eq_eta_update}
\end{alignat}
\end{theorem}

\begin{proof}
\item
We first note that the Lagrange multiplier update steps (\ref{th:eq_kappa_update}) and (\ref{th:eq_eta_update}) are trivially equivalent since it results directly from the definitions of $\kappa_i$ and $\eta_i$ and $\tilde{z}$.
\paragraph{Lagrangian minimization (\ref{th:eq_lagrangian_minimization}).}
We now show that the minimization or the \textit{Constrained ADMM} Lagrangian can be rewritten to $N$ minimizations of the \textit{Distributed Augemented Lagrangian}.

Since $\chi(y^k) = 0$, the \textit{Constrained ADMM} Lagrangian minimization (\ref{th:eq_lagrangian_minimization}) step can be simplified to:
\begin{align*}
z^{k+1} := \min_z f(z) + \kappa^k \cdot h(z) + \frac{\nu}{2} \norm{h(z)}^2 + \eta^k \cdot (z - y^k) + \frac{\rho}{2} \norm{z - y^k}^2.
\end{align*}
Using the defitions of $f$, $h$, $z$ we can fully separate this expression as a sum of $N$~terms:
\begin{align*}
(z_0, .., z_{N-1})^{k+1} := \min_{z_0, .., z_{N-1}} \sum_i {f_i(z_i) + \kappa_i^k \cdot h_i(z_i) + \frac{\nu}{2} \norm{h_i(z_i)}^2 + \eta_i^k \cdot (z_i - y^k) + \frac{\rho}{2} \norm{z_i - y^k}^2}.
\end{align*}
The terms of the sum are independent from each other, since each depends only on $z_i$, the other variables are constants throughout the minimization. In other words, each term of the sum can be minimized independently, such that one can rewrite it as:
\begin{align*}
z_i^{k+1} &:= \min_{z_i} { \left( f_i(z_i) + \kappa_i^k \cdot h_i(z_i) + \frac{\nu}{2} \norm{h_i(z_i)}^2 + \eta_i^k \cdot (z_i - y^k) + \frac{\rho}{2} \norm{z_i - y^k}^2 \right) },
\end{align*}
which are the $N$ minimizations of \textit{Distributed Augmented Lagrangain} of the sub-problems:
\begin{align*}
z_i^{k+1} &:= \min_{z_i} L_{i, \nu, \rho}(z_i, y^k, \kappa^k, \eta^k), 
\end{align*}
which is the first step of the \textit{Decentralized Augmented Lagrangian}~(\ref{eq:dec-algo-newton}).

\paragraph{Consensus variable update (\ref{th:eq_y_update}).}
We now prove that minimizing the \textit{Constrained ADMM} Lagrangian over $y$ corresponds to a consensus variable update with the average of the local variables $z_i$.

The step (\ref{th:eq_y_update}) of the \textit{Constrained ADMM} algorithm is a minimization over $y$ of the Lagrangian:
\begin{align*}
y^{k+1} := \min_y \left( f(z^{k+1}) + \chi(y) + \kappa^k \cdot h(z^{k+1}) + \frac{\nu}{2} \norm{h(z^{k+1})}^2 + \eta^k \cdot (z^{k+1} - y) + \frac{\rho}{2} \norm{z^{k+1} - y}^2 \right),
\end{align*}
First, we remove from the expression the terms that are not depending on $y$, i.e. $f(z^{k+1})$, $h(z^{k+1})$ and $\eta^k \cdot z^{k+1}$ such that it gives:
\begin{align*}
y^{k+1} := \min_y \left( \chi(y) - \eta^k \cdot y + \frac{\rho}{2} \norm{z^{k+1} - y}^2 \right).
\end{align*}
We proved earlier that $\chi(y) = 0$, and we can rewrite the above expression as a minimization over $\tilde{z}$ and without the term $\chi(y)$ since it is zero:
\begin{align*}
\tilde{z}^{k+1} := \min_{\tilde{z}} \left( - \eta^k \cdot y + \frac{\rho}{2} \norm{z^{k+1} - y}^2 \right),
\end{align*}
which gives the following expression when using the variables $\eta_i$ and $\tilde{z}$ instead of the stacked $\eta$ and $z$:
\begin{align*}
\tilde{z}^{k+1} := \min_{\tilde{z}} \left( - \sum_i{\eta_i^k \cdot \tilde{z}} + \frac{\rho}{2} \sum_i \norm{z_i^{k+1} - \tilde{z}}^2 \right).
\end{align*}
Since the above expression is convex w.r.t. $\tilde{z}$, a necessary and sufficient condition for $\tilde{z}^{k+1}$ to be a minimum is that the gradient is zero in $\tilde{z}^{k+1}$:
\begin{align}
- \sum_i{\eta_i^k} + \frac{\rho}{2} \sum_i 2 (z_i^{k+1} - \tilde{z}^{k+1}) = 0, \label{eq:optimality_condition_second_minimization}
\end{align}
which can be rewritten as follows, when moving $\tilde{z}^{k+1}$ out of the sum, and gathering the terms $z_i^{k+1}$ and $\eta_i^k$ together:
\begin{align*}
- \rho N \tilde{z}^{k+1} + \rho \sum_i (z_i^{k+1} - \frac{\eta_i^{k}}{\rho}) = 0,
\end{align*}
which leads to:
\begin{align}
\tilde{z}^{k+1} = \frac{1}{N} \sum_i (z_i^{k+1} - \frac{\eta_i^{k}}{\rho}).
\end{align}

This expression can be simplified further by using the fact that $\sum_i{\eta_i^k} = 0$ after the first iteration. This is indeed proven straightforwardly by injecting the update rule $\eta_i^{k+1} = \eta_i^k + \rho (z_i^{k+1} - 
\tilde{z}^{k+1})$ in \ref{eq:optimality_condition_second_minimization}. The update rule therefore becomes 
\begin{align*}
\tilde{z}^{k+1} = \frac{1}{N} \sum_i z_i^{k+1},
\end{align*}
which is the consensus variable update step of the \textit{Distributed Augmented Lagrangian}~(\ref{eq:dec-z_update}).
\end{proof}
